# Supplementary material for: Efficacy of face coverings in reducing transmission of COVID-19: calculations based on models of droplet capture
Source: arXiv:2008.04995 source file (2021-04-03)
Supplement: Supplementary file 1 [file supplementary.pdf]

# Supplementary Material for "Efficacy of face coverings in reducing transmission of COVID-19: calculations based on models of droplet capture"

## I. EXPLICIT KUWABARA FLOW FIELD PARAMETERS

The components of velocity (3) in plane polar coordinates are

$$u_\rho = \mathbf{u} \cdot \mathbf{e}_\rho = \cos\theta \frac{f(\rho)}{\rho}, \tag{S1a}$$

$$u_\theta = \mathbf{u} \cdot \mathbf{e}_\theta = -\sin\theta f'(\rho). \tag{S1b}$$

The vorticity is

$$\boldsymbol{\omega} = \boldsymbol{\nabla} \times \mathbf{u} \tag{S2}$$

The outer boundary conditions introduced in section III A 1 can be expressed as

$$f(\rho_b) = \rho_b, \tag{S3a}$$

$$f(\rho_b) - \rho_b f'(\rho_b) - \rho_b^2 f''(\rho_b) = 0, \tag{S3b}$$

where $\rho_b = a_f/\sqrt{\alpha}$ is the location of the outer boundary. Together with the inner boundary conditions $f(a_f) = 0$ (no penetration) and $f'(a_f) = 0$ (no slip) we obtain the solution for the coefficients in (4b) as

$$f_1 = \frac{2-\alpha}{4K} a_f^2 \tag{S4a}$$

$$f_2 = \frac{\alpha - 1}{2K} \tag{S4b}$$

$$f_3 = -\frac{\alpha}{4a_f^2 K} \tag{S4c}$$

$$f_4 = \frac{1}{K} \tag{S4d}$$

introducing the hydrodynamic factor:

$$K = -\frac{\ln\alpha}{2} - \frac{3}{4} + \alpha - \frac{\alpha^2}{4}. \tag{S4e}$$

This flow field was first obtained by Kuwabara[1], from whom it bears its name.

## II. LATTICE BOLTZMANN SIMULATIONS OF FLOW FIELD AROUND FIBRES

Lattice Boltzmann (LB) simulations are performed on a two-dimensional lattice of $n_x$ by $n_y$ lattice sites; $x$ is the flow direction. Our code is a modified version of a Python code of the Palabos group at the University of Geneva[2]. Their code models flow around a cylinder.

The lattice is the standard square D2Q9 lattice with nine velocities at each lattice site[3–5], each pointing along a vector $\mathbf{e}_i$. The vectors $\mathbf{e}_i = (0,0)$, $(0,-1)$, $(0,1)$, $(-1,0)$, $(-1,-1)$, $(-1,1)$, $(1,0)$, $(1,-1)$, $(1,1)$. The LB fluid has only one parameter, its relaxation rate $\tau$. This controls the LB dynamics via

$$f_i(\mathbf{r} + \mathbf{e}_i, t+1) = f_i(\mathbf{r}, t) - \tau^{-1}\left[f_i(\mathbf{r}, t) - f_{eq,i}(\mathbf{r}, t)\right] \tag{S5}$$

for $f_i(\mathbf{r}, t)$ the density at site $\mathbf{r}$ and time $t$, associated with flow in direction $i$. The density $\rho_{LB} = \sum_i f_i$, and the flow velocity $\mathbf{u} = \rho_{LB}^{-1}\sum_i f_i \mathbf{e}_i$. The LB gas is compressible, so the density $\rho_{LB}$ does vary with position but at the small Reynolds numbers we run for, this variation is small. We start with an initial density $\rho_{LB} = 1$. The equilibrium density is

$$f_{eq,i}(\mathbf{r}, t) = \rho_{LB} w_i \left[1 + 3\mathbf{e}_i.\mathbf{u}\right] \tag{S6}$$

with weights $w_i = (4/9, 1/9, 1/9, 1/9, 1/36, 1/36, 1/9, 1/36, 1/36)$.

The LB's relaxation time $\tau$ sets the LB kinematic viscosity, via $\nu_{LB} = (2\tau - 1)/6$[5]. We set $\tau = 1$ in LB units. This sets its kinematic viscosity to be $\nu_{LB} = 1/6$ in LB units. The LB method suffers from stability issues outside of a relatively narrow range of values of $\tau \lesssim 1$[4]. We compared $\lambda$ values for $\tau = 0.75$ and $\tau = 1$, and there were only very small differences.

We run the LB simulations until the change in mean flow speed along $x$ is very small. We then take that flow field as being a steady-state flow field, and use it to evaluate particle trajectories.

### A. Boundary conditions

We have periodic boundary conditions along the direction perpendicular to flow ($y$). Along the downstream edge along $x$, we impose continuity of the missing components. The three missing components are the ones pointing upstream (because in the bulk these are propagated from the line of elements downstream which are missing along this edge). We simply set the values along the final row equal to their known values along the last-but-one row. As this downstream of the fibres, we expect this boundary to have little effect on our results.

#### 1. Zou-He boundary conditions

To impose the flow field, we use standard Zou-He boundary conditions[3] along the upstream, $x = 0$ edge of the simulation box. To do this, we first impose velocity along left-edge lattice sites, at $u_x = u_{BC}$ and $u_y = 0$, then within Zou He boundary conditions, the density is calculated from

$$\rho = \frac{1}{1-u}\left[f_0 + f_1 + f_2 + 2\left(f_3 + f_4 + f_5\right)\right] \tag{S7}$$

note the first three $f$s are those corresponding to a zero $x$ component $\mathbf{e}_i$, while the second three are the ones with negative $x$ components. We then set the three $f$s with positive $x$ components

$$f_6 = f_3 + \frac{2}{3}\rho u_{BC} \tag{S8}$$

$$f_7 = f_5 + \frac{1}{2}\left(f_2 - f_1\right) \tag{S9}$$

$$f_8 = f_4 - \frac{1}{2}\left(f_2 - f_1\right) \tag{S10}$$

#### 2. Fibres

A fibre is modelled as a circular domain of all lattice sites within a radius $r_{LB}$ of the fibre centre. So the simulation lattice has two types of sites, air sites plus fibre sites. The boundary conditions on the fibres are standard LB on-site bounce back[5,6], to model stick boundary conditions. So at every step the velocities in all fibre sites are reversed.

The fibre radius is the lengthscale we use to define the Reynolds number in our simulation, via $\mathrm{Re} = u_{BC} r_{LB}/\nu_{LB} < 1$.

### B. Model mask

We model the fibres as a disordered hexagonal lattice of discs, each of the same radius $r_{LB}$, see Fig. S1(b). The lattice constant of the hexagonal lattice is $a$, and so the fibres occupy an area fraction, $\alpha = (\pi\sqrt{3.0}/6)(2r/a)^2$. The disordered lattice is obtained by starting with a perfectly ordered hexagonal lattice, then displacing the centre of a disc randomly and uniformly within a square of side $r_{\mathrm{disp}}$ centred at the position in the perfect lattice.

Note that in a perfect lattice some streamlines periodically repeat along with the lattice and simulations of particles with low Stokes number are then also periodic and so are not filtered out, no matter how many layers there are in the lattice. As the fibres in masks are not perfectly ordered, this is unrealistic, and so we introduce the disorder.

### C. A fibre for calculation of $\lambda$

We cannot have an isolated single fibre in two dimensions due to the Stokes paradox. So, we simulate in effect a single row of fibres perpendicular to the flow direction, with a spacing of the lattice constant $a$. This is shown in Fig. S1(a). The system has two fibres, one in the centre (along $y$) for the calculation of $\lambda$ and another at the edge. Thus it should be borne in mind that our "single-fibre" is a fibre in an array of a set density, and that this density affects the flow field.

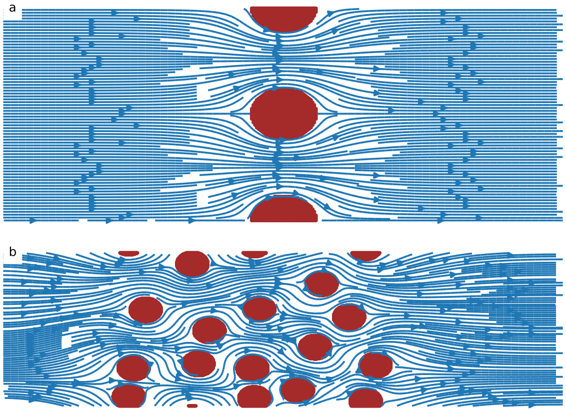


FIG. S1. Flow fields calculated using Lattice-Boltzmann simulations. The flow field is shown via (blue) streamlines, with the fibres shown in dark red. The system is periodic along $y$. (a) is the system used to calculate the single-fibre $\lambda$ for $\alpha = 0.2$, the fibre spacing is $d_f/\sqrt{\alpha}$. (b) is a model filter, made up five layers of a disordered hexagonal lattice of fibres, with the same $\alpha$. $U_0 = 2.7\,\mathrm{cm\,s^{-1}}$, and $d_f = 15\,\mu\mathrm{m}$, with the lattice constant equal to $0.375\,\mu\mathrm{m}$ so fibres are 40 LB lattice sites across. Note (a) is shown at a larger scale than (b), in both systems the fibres are the same size in LB units.

### D. Test of assumption that fibres filter independently

Equation 13 was derived assuming that the fibres filter independently, and each fibre's local environment is well-described by the same $\alpha$. This can only be approximately true, so we tested it using LB simulations. We calculated the single-fibre $\lambda$ using a system as shown in Fig. S1(a), and also computed the penetration directly using a model filter composed of five layers of a disordered hexagonal lattice of fibres, using a system as shown in Fig. S1(b).

### E. Particle trajectories

Once we have a steady-state flow-field, we simulate (independent) particle trajectories in this flow field, to estimate the $\lambda$ or filtration efficiency.

Each particle's trajectory is obtained by starting the particle at a point at $x = 0$, and at a selected $y$ coordinate. The particle's initial velocity is that of the flow field.

The only force on the particle is Stokes drag from the flow field. Therefore its acceleration obeys (6). The particles are not on a lattice but the flow field is only defined on the lattice of the LB simulations. Thus the flow field at the centre of the particle $\mathbf{u}(\mathbf{r})$ is obtained from bilinear interpolation of the surrounding four lattice sites of the LB flow field.

We then integrate the trajectory forward in time, using modified Euler integration, until the particle either collides with a fibre, or reaches the right-hand (large $x$) edge of the simulation box. At each time step, we check for a collision. A collision occurs if the centre of the particle is within the sum of the radii of the fibre and particle.

### 1. Evaluation of $\lambda$ from Lattice Boltzmann flow field

The single-fibre $\lambda$ is determined by starting with a pair of initial positions along $y$ that bracket the value of $y$ that separates where particle trajectories collide with the fibre and where the particle passes by the fibre. One initial position is the $y$ coordinate of the centre of the fibre and the second is sufficiently far away that trajectory misses the fibre. Then a bisection search is performed to accurately determine where the dividing $y$ is for collisions. $\lambda$ is then just twice this $y$ value; the collision zone is symmetric around the centre of the central fibre as the simulation box is symmetric, see Fig. S1(a).

### 2. Evaluation of penetration of model filter from Lattice Boltzmann flow field

The penetration for a model mask is determined by starting a set of $N_{\mathrm{samp}}$ particles on an evenly-spaced grid along the $y$ axis. Then particle trajectories are calculated, and the penetration is estimated from the fraction of particles that penetrate the model filter.

## III. SCANNING ELECTRON MICROSCOPE IMAGES

Unless otherwise stated, SEM images feature a 100 µm scalebar. Macroscopically, the inner layer of both N95/FFP2 respirators and one of the KN95 respirators appeared to consist of a single layer; however, under SEM imaging we found two distinct populations of fibre sizes on opposing sides of the sample which we treat as two fused layers. We number these layers 1 and 2 for the innermost and outermost inner layers respectively. The distribution of fibre sizes determined from these images (and additional images not shown) are shown in Fig. S2. The parameters of the log-normal fits to these size distributions, as well as the measured material properties (thickness and volume fraction) are given in table S1. In table S2 we show the results show the results of the indirect method (described in the main text) of *inferring* the fabrics' material properties from the yarn measurements for two of the woven fabrics; note that this method predicts thinner (and thus denser) fabrics.

N95/FFP2 Respirator 1:

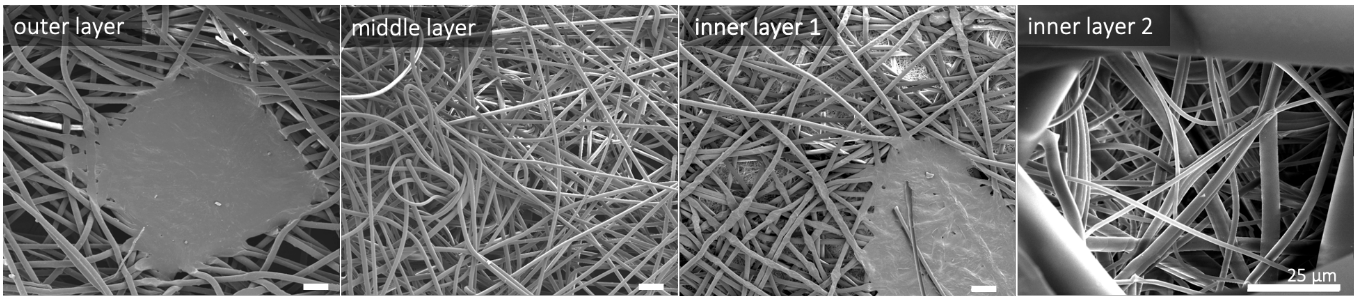


N95/FFP2 Respirator 2:

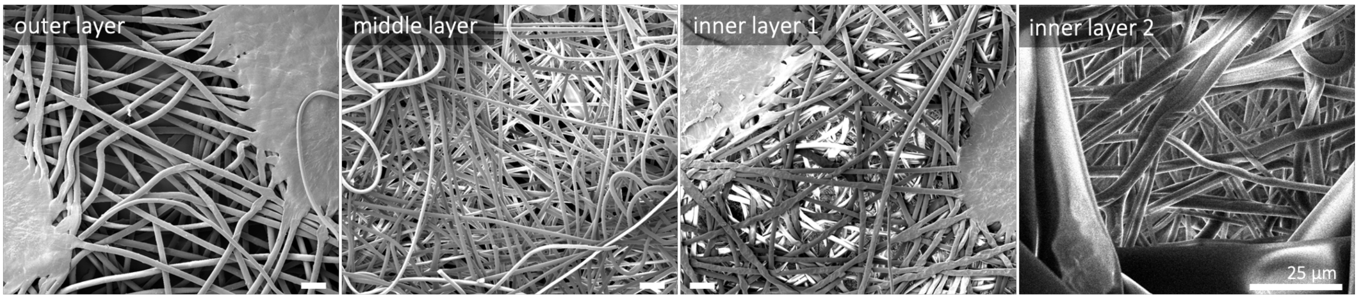


KN95 Respirator 1:

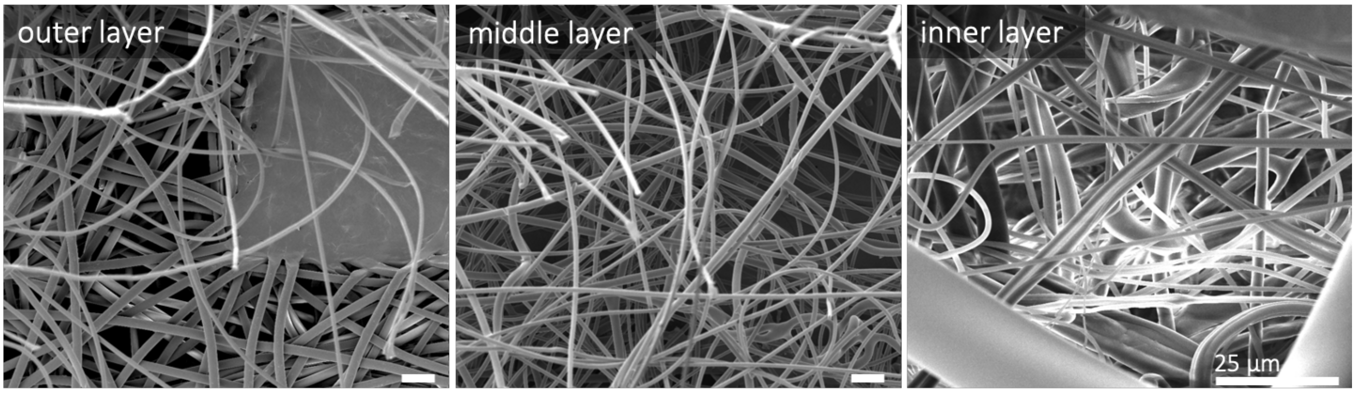


KN95 Respirator 2:

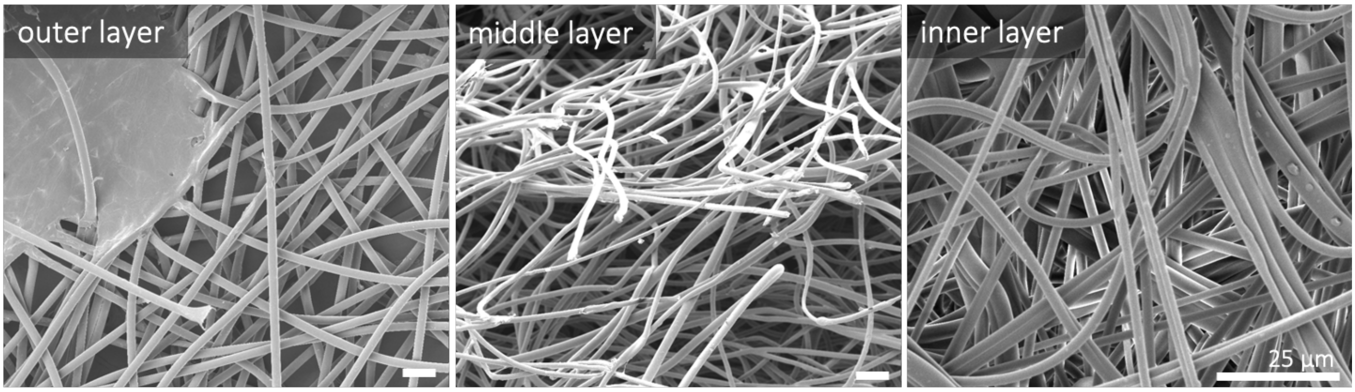

Surgical masks (labelled SM4 and SM5 in main text):

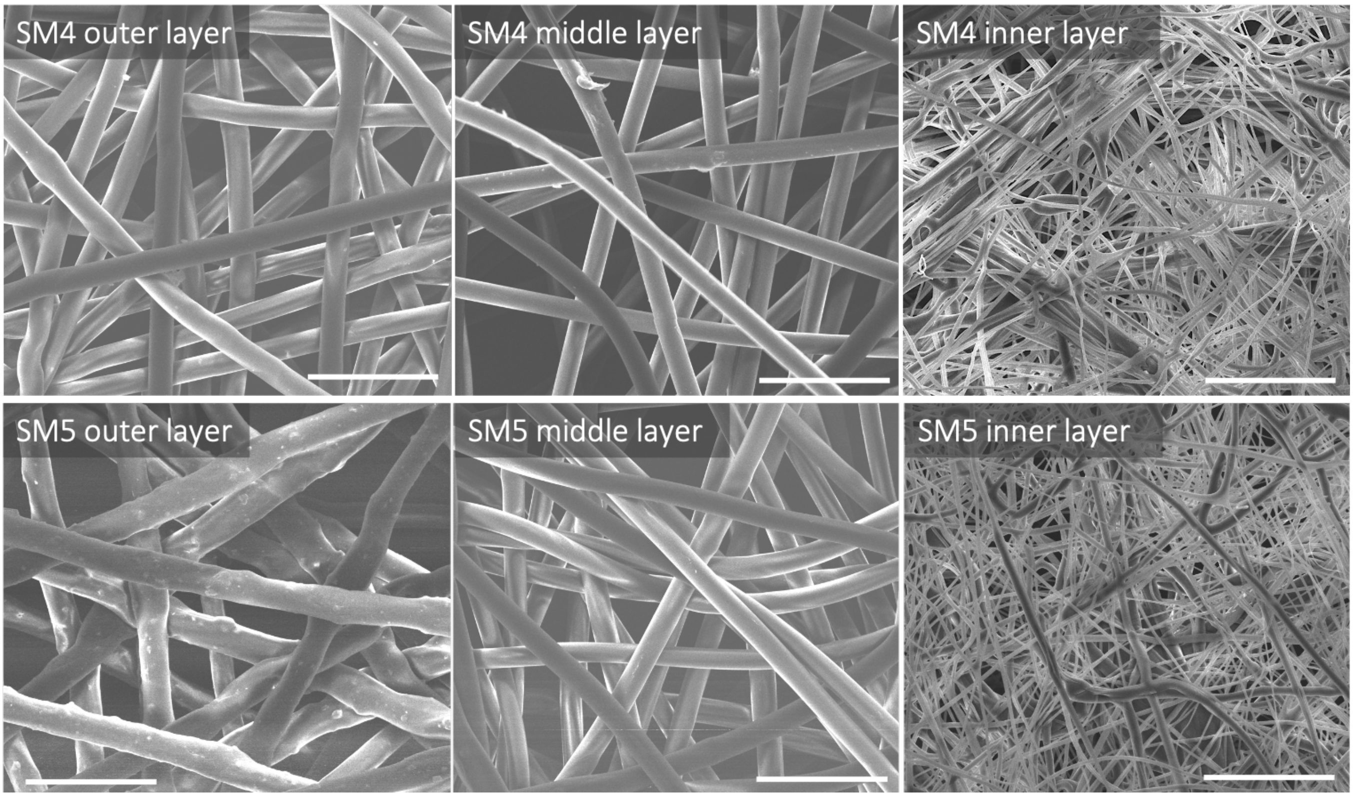


3-layered cotton mask:

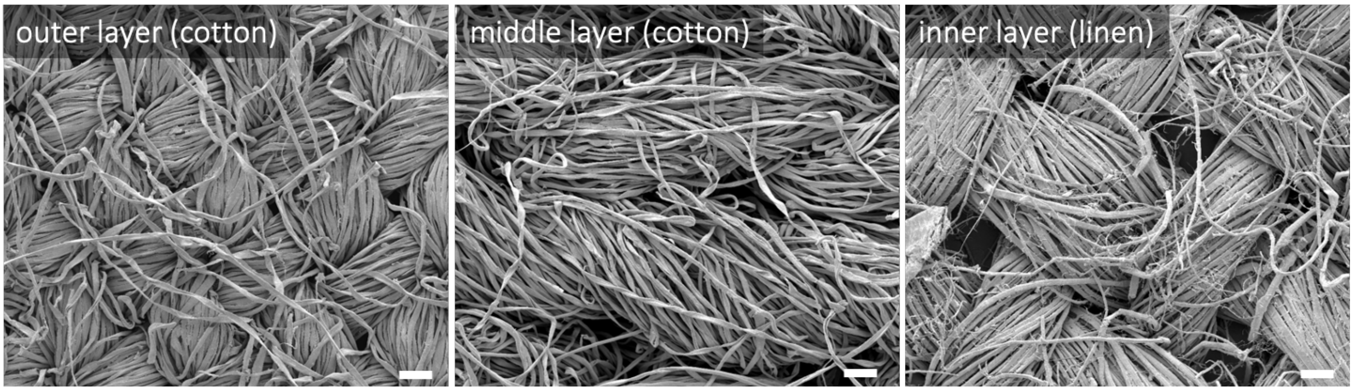


Woven fabrics:

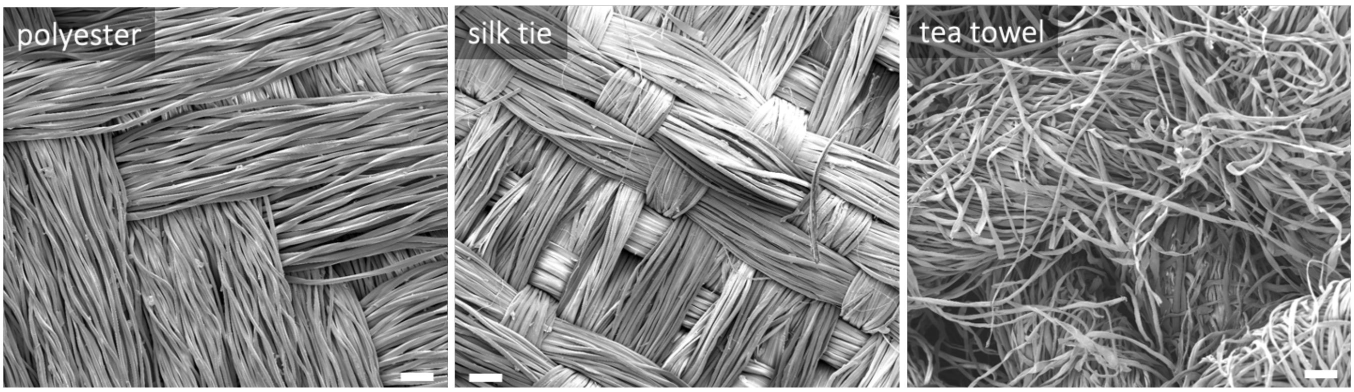

Knitted fabrics:

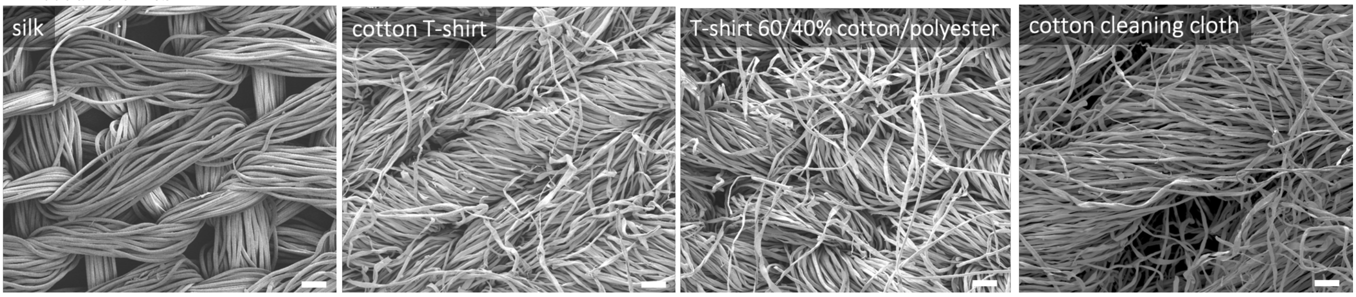


Nonwoven fabrics:

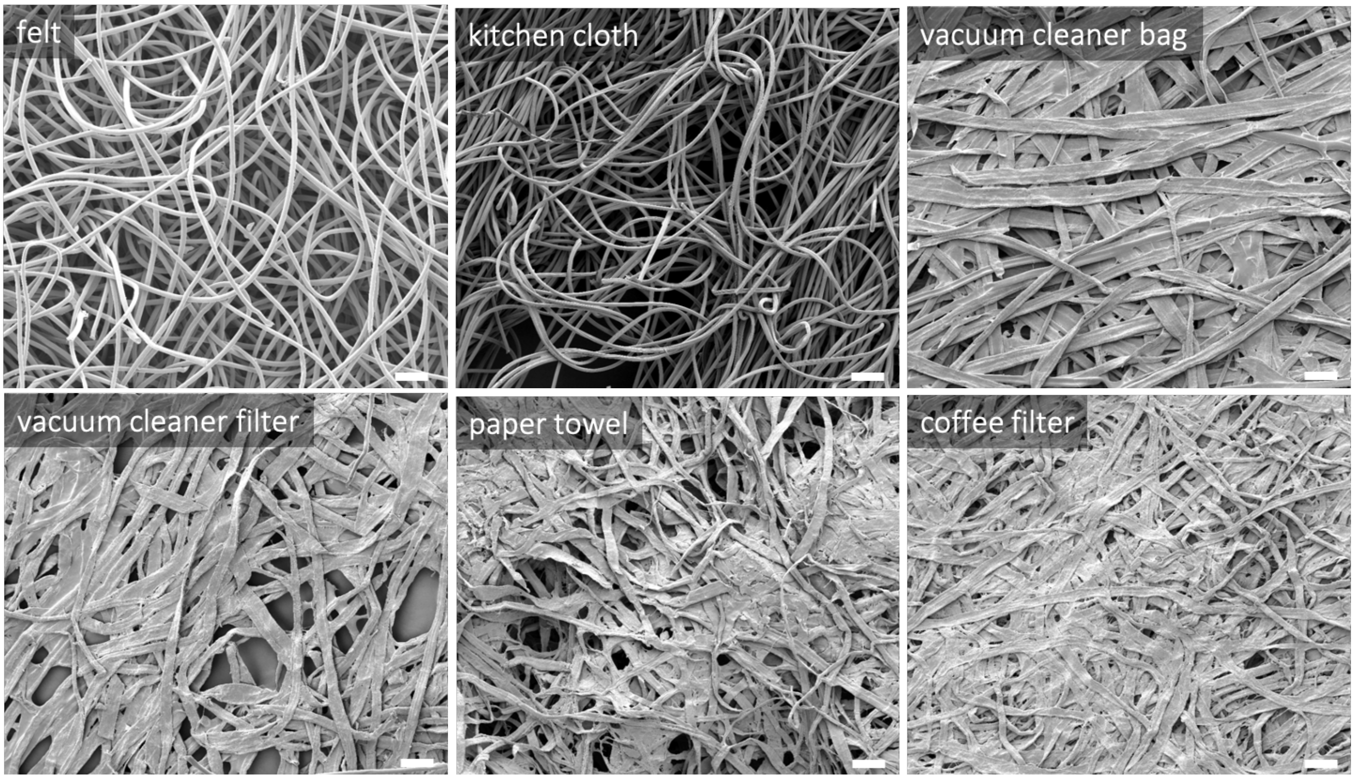


## IV. DIFFUSION COLLECTION EFFICIENCY

To model the effect of diffusion we use the result of Stechkina and Fuchs[7]:

$$\frac{\lambda_D}{d_f} = \frac{2.9}{(K\mathrm{Pe}^2)^{1/3}} + \frac{0.624}{\mathrm{Pe}} + \frac{1.24R^{2/3}}{\sqrt{K\mathrm{Pe}}}, \tag{S11}$$

where $R = d_p/d_f$, and $K$ is given by (S4e) — this expression assumes the Kuwabara flow field. Note that the Péclet number scales as $\mathrm{Pe} \propto d_f$ (see definition (12) in the main text) which must be taken into consideration when averaging over a polydisperse system of fibres.

## V. ELECTROSTATIC POTENTIAL AROUND CYLINDRICAL FIBRES

The electric potential of a line charge (monopole) of magnitude $\Lambda$ centred at the origin is

$$\Phi_0 = -\frac{\Lambda}{2\pi\epsilon_0} \ln\left(\frac{\rho}{\rho_0}\right) \tag{S12}$$

where $\rho_0$ is a reference point close to the line charge where we set the potential to zero, and $\epsilon_0$ is the vacuum permittivity. This generalises to assemblies of line charges on the fibre surface $\rho = a_f$ via a multipole expansion of

| fabric | type | material | bulk density (g/cm$^3$) | $\mu_{d_f}$ | $\sigma_{d_f}$ | $L_x$ (mm) | $\alpha$ |
|---|---|---|---|---|---|---|---|
| N95/FFP2 respirator 1 inner layers | respirator | polypropylene | 0.91 | - | - | 0.448 | 0.087 |
| N95/FFP2 respirator 1 inner layer 1 | - | - | - | 0.375 | 0.189 | - | - |
| N95/FFP2 respirator 1 inner layer 2 | - | - | - | 2.987 | 0.074 | - | - |
| N95/FFP2 respirator 1 middle layer | respirator | polypropylene | 0.91 | 2.807 | 0.145 | 0.663 | 0.114 |
| N95/FFP2 respirator 1 outer layer | respirator | polypropylene | 0.91 | 3.238 | 0.104 | 0.944 | 0.101 |
| N95/FFP2 respirator 2 inner layers | respirator | polypropylene | 0.91 | - | - | 0.595 | 0.069 |
| N95/FFP2 respirator 2 inner layer 1 | - | - | - | 0.733 | 0.378 | - | - |
| N95/FFP2 respirator 2 inner layer 2 | - | - | - | 3.023 | 0.066 | - | - |
| N95/FFP2 respirator 2 middle layer | respirator | polypropylene | 0.91 | 2.738 | 0.140 | 0.796 | 0.104 |
| N95/FFP2 respirator 2 outer layer | respirator | polypropylene | 0.91 | 3.220 | 0.109 | 0.994 | 0.097 |
| KN95 respirator 1 inner layer | respirator | polypropylene | 0.91 | 0.375 | 0.189 | 0.814 | 0.106 |
| KN95 respirator 1 middle layer | respirator | polypropylene | 0.91 | 2.683 | 0.311 | 2.003 | 0.026 |
| KN95 respirator 1 outer layer | respirator | polypropylene | 0.91 | 3.200 | 0.285 | 0.547 | 0.110 |
| KN95 respirator 2 inner layer | respirator | polypropylene | 0.91 | 0.733 | 0.378 | 0.581 | 0.057 |
| KN95 respirator 2 middle layer | respirator | polypropylene | 0.91 | 2.828 | 0.211 | 1.902 | 0.026 |
| KN95 respirator 2 outer layer | respirator | polypropylene | 0.91 | 3.268 | 0.048 | 0.996 | 0.131 |
| SM4 inner layer | surgical mask | polypropylene | 0.91 | 0.980 | 0.410 | 0.430 | 0.051 |
| SM4 middle layer | surgical mask | polypropylene | 0.91 | 2.780 | 0.051 | 0.294 | 0.070 |
| SM4 outer layer | surgical mask | polypropylene | 0.91 | 2.898 | 0.056 | 0.214 | 0.082 |
| SM5 inner layer | surgical mask | polypropylene | 0.91 | 0.822 | 0.497 | 0.240 | 0.080 |
| SM5 middle layer | surgical mask | polypropylene | 0.91 | 2.861 | 0.065 | 0.241 | 0.094 |
| SM5 outer layer | surgical mask | polypropylene | 0.91 | 3.033 | 0.080 | 0.358 | 0.063 |
| cloth mask inner layer | woven | linen | 1.50 | 2.571 | 0.356 | 1.200 | 0.079 |
| cloth mask middle layer | knitted | cotton | 1.54 | 2.714 | 0.248 | 2.300 | 0.149 |
| cloth mask outer layer | woven | cotton | 1.54 | 2.775 | 0.282 | 1.027 | 0.077 |
| tie 1 | woven | polyester | 1.38 | 2.682 | 0.269 | 0.825 | 0.138 |
| tie 2 | woven | silk | 1.33 | 2.578 | 0.152 | 0.340 | 0.263 |
| tea towel | woven | cotton | 1.54 | 2.594 | 0.354 | 2.017 | 0.073 |
| shirt | knitted | silk | 1.33 | 2.780 | 0.079 | 0.804 | 0.088 |
| t-shirt 1 | knitted | cotton | 1.54 | 2.703 | 0.358 | 0.960 | 0.120 |
| t-shirt 2 | knitted | 60% cotton 40% polyester | 1.476 | 2.759 | 0.287 | 0.814 | 0.138 |
| cleaning cloth | knitted | cotton | 1.54 | 2.549 | 0.396 | 2.673 | 0.072 |
| felt | nonwoven | felt | 1.50 | 2.664 | 0.113 | 1.692 | 0.077 |
| all purpose kitchen cloth | nonwoven | 70% viscose 30% PET | 1.534 | 2.490 | 0.128 | 0.442 | 0.069 |
| vacuum cleaner bag | nonwoven | paper (cellulose) | 1.50 | 3.427 | 0.484 | 0.064 | 0.202 |
| vacuum cleaner filter | nonwoven | paper (cellulose) | 1.50 | 3.379 | 0.332 | 0.228 | 0.179 |
| paper towel | nonwoven | paper (cellulose) | 1.50 | 3.031 | 0.400 | 0.477 | 0.062 |
| coffee filter | nonwoven | paper (cellulose) | 1.50 | 3.253 | 0.263 | 0.114 | 0.293 |

TABLE S1. Measured properties of sample masks. The manufacturer did not state what material the surgical masks and respirators were made of, so we assigned polypropylene to them as our best guess. For the 60 % cotton t-shirt we state the results for the first (most likely cotton) peak. Parameters are shown for the distribution of fibre diameters modelled by the log-normal $\ln(d_f/\mu\text{m}) \sim \mathcal{N}(\mu_{d_f}, \sigma_{d_f}^2)$; the modal diameter in µm is given by $\exp(\mu_{d_f})$.

| fabric | type | $D_x$ | $D_y$ | $l_x$ | $l_y$ | $\langle L_x \rangle$ (mm) | $\langle \alpha \rangle$ |
|---|---|---|---|---|---|---|---|
| cloth mask inner layer | linen | 0.36 | 0.36 | 0.54 | 0.55 | 0.47 | 0.20 |
| cloth mask outer layer | cotton | 0.25 | 0.21 | 0.31 | 0.25 | 0.38 | 0.22 |

TABLE S2. Estimating the properties of two sampled woven fabrics using an indirect method described in the main text (cf. discussion around (17). Here we estimated the warp and weft widths ($D_x$ and $D_y$) from SEM images, whereas we estimated the separations between their centres ($l_x$ and $l_y$) from optical microscopy taking advantage of the larger field of view. The parameters $\langle L_x \rangle$ and $\langle \alpha \rangle$ are inferred from the yarn parameters ($D_x$, $D_y$, $l_x$ and $l_y$). Note that this method predicts a thinner (and thus more dense) fabric than was determined by optical microscopy in table S1.

$\ln(\rho/\rho_0)$[8]. For surface line charge distributions of the form $\sigma = \sigma_0 \cos(k\theta)$ we find the electric potential outside the fibre adopts the form

$$\Phi_k = \frac{\sigma_0 a_f^{k+1} \cos(k\theta)}{\epsilon_0 (1+\epsilon_f) k \rho^k}$$

for $k > 0$ and $\rho > a_f$ and where $\epsilon_f$ is the dielectric constant of the fibre. For electret fibres the most important terms from this expansion are the monopole term (S12) for fibres with net charge, or the $k = 1$ term

$$\Phi_1 = \frac{\sigma_0 a_f^2 \cos\theta}{\epsilon_0 (1+\epsilon_f) \rho} \tag{S13}$$

for fibres with a dipole polarisation.

Dielectric breakdown is expected to occur where the field $|\Phi'(a_f)| = 3 \times 10^6\,\mathrm{V\,m^{-1}}$, the dielectric strength of air. This corresponds to surface charges of $\sigma_0 \sim 3\,\mathrm{nC\,cm^{-2}}$ for monopole fibres and $\sigma_0 \sim (1+\epsilon_f)3\,\mathrm{nC\,cm^{-2}}$ for dipolar fibres. Polypropylene, a widely used material for the electret fibres in respirators, has $\epsilon_f \simeq 2$ giving $\sigma_0 \sim 9\,\mathrm{nC\,cm^{-2}}$. Electret fibres can readily sustain charges in the $\mathcal{O}(1\,\mathrm{nC\,cm^{-2}})$ range[9,10], so they are close to this upper limit.

Natural cellulose fabrics such as cotton and wool can typically sustain a maximum charge density in the range of $\mathcal{O}(0.01\,\mathrm{nC\,cm^{-2}})$ (or $\mathcal{O}(0.1\,\mathrm{nC\,cm^{-2}})$ for silk) when charged tribolectrically[11]. This is one to two orders of magnitude smaller than in electret fibres, so we expect electromagnetic forces to be negligible in cloth fabrics compared to respirators.


[1] S. Kuwabara, "The Forces experienced by Randomly Distributed Parallel Circular Cylinders or Spheres in a Viscous Flow at Small Reynolds Numbers," J. Phys. Soc. Jpn. **14**, 527–532 (1959).

[2] "Palabos - university of geneva," (2020).

[3] Q. Zou and X. He, "On pressure and velocity boundary conditions for the lattice boltzmann bgk model," Physics of Fluids **9**, 1591–1598 (1997).

[4] O. Behrend, R. Harris, and P. B. Warren, "Hydrodynamic behavior of lattice Boltzmann and lattice Bhatnagar-Gross-Krook models," Phys. Rev. E **50**, 4586–4595 (1994).

[5] Y. B. Bao and J. Meskas, *Lattice Boltzmann method for fluid simulations* (Department of Mathematics, Courant Institute of Mathematical Sciences, New York University, New York, 2011).

[6] D. P. Ziegler, "Boundary conditions for lattice Boltzmann simulations," J Stat Phys **71**, 1171–1177 (1993).

[7] I. B. Stechkina and N. A. Fuchs, "Studies on Fibrous Aerosol Filters—I. Calculation of Diffusional Deposition of Aerosols in Fibrous Filters," Ann. Occup. Hyg. (1966), 10.1093/annhyg/9.2.59.

[8] D. J. Griffiths, *Introduction to Electrodynamics*, fourth edition ed. (Cambridge University Press, Cambridge, United Kingdom ; New York, NY, 2018).

[9] C. C. Chen, M. Lehtimäki, and K. Willeke, "Loading and filtration characteristics of filtering facepieces," Am. Ind. Hyg. Assoc. J. **54**, 51–60 (1993).

[10] A. Kravtsov, H. B. Nig, S. Zhandarov, and R. Beyreuther, "The electret effect in polypropylene fibers treated in a corona discharge," Adv. Polym. Technol. **19**, 5 (2000).

[11] S. Liu, W. Zheng, B. Yang, and X. Tao, "Triboelectric charge density of porous and deformable fabrics made from polymer fibers," Nano Energy **53**, 383–390 (2018).

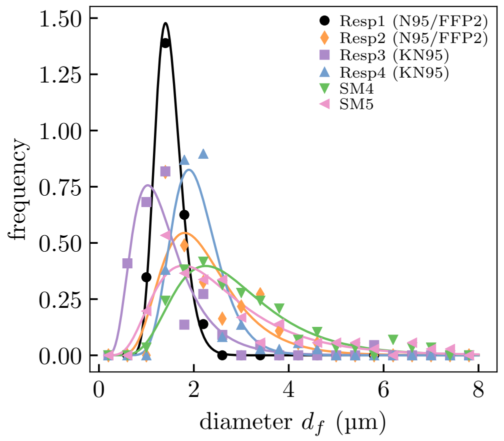


(a) Innermost mask layers

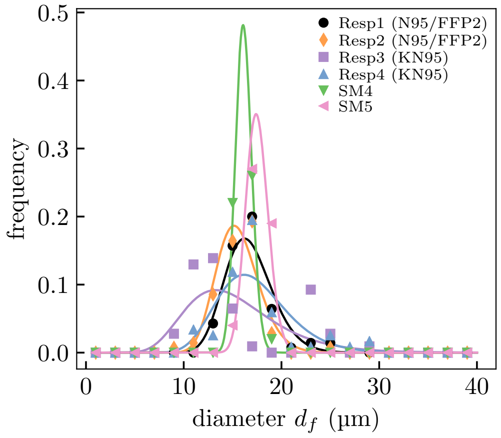


(b) Middle mask layers

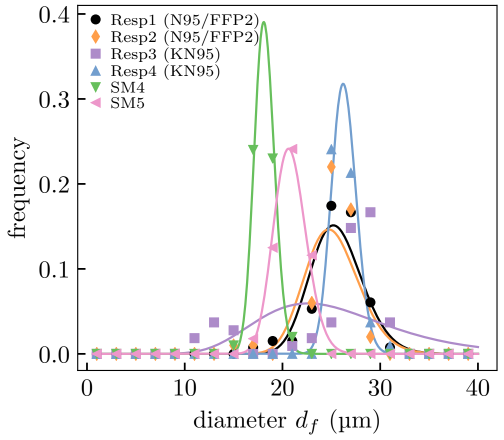


(c) Outer mask layers

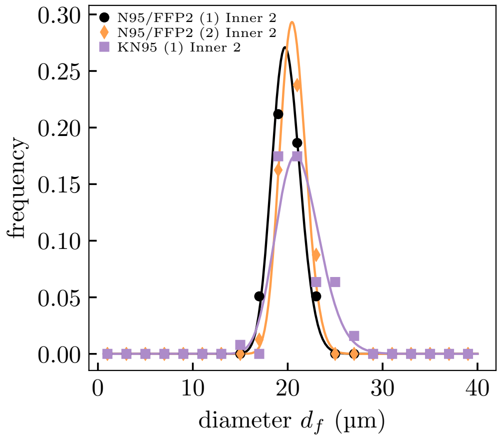


(d) Other mask layers

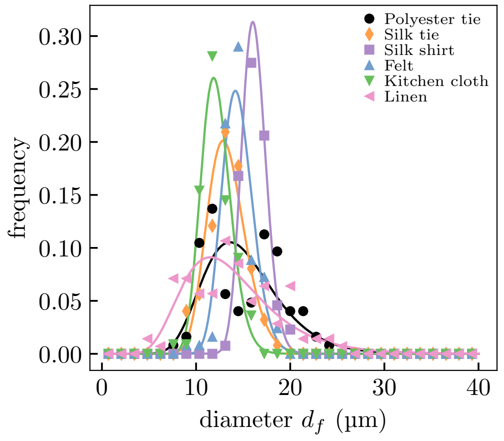


(e) Other fabrics

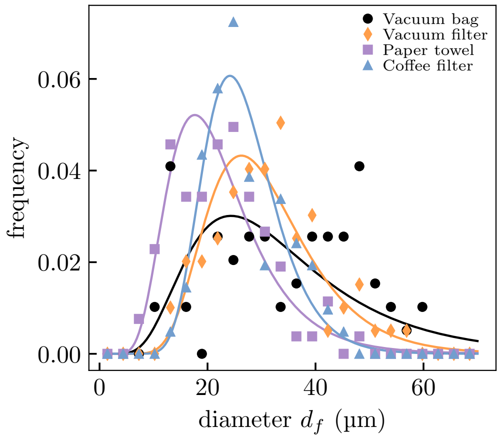


(f) Paper samples

FIG. S2. Distribution of fibre diameters in sampled fabric layers determined from analysis of SEM images (points) and their log-normal fits (lines). Mask layers are grouped by those with similar size distributions. (a-d) Sampled masks show progressively smaller fibres as they move innerwards; this is true for all surgical masks (SM), respirators (Resp) and the (cotton/linen) cloth mask sampled. Panel (a) shows that the innermost layer was particularly fine in all cases, containing fibres an order of magnitude smaller in the $\mathcal{O}(1\,\mu\mathrm{m})$ range. (e) Other fabric samples showed fibres of comparable diameter (10 to 20 µm) and polydispersity to those in sampled masks (and cotton samples shown in Fig. 1 in the main text), suggesting they could be used as substitute materials in homemade masks. (f) Paper samples contained the largest and most polydisperse fibres, suggesting they would have worse filtration performance than the cloth layers sampled.
